# Supplementary material for: Neutrino Flux Predictions for the NuMI Beam
Source: arXiv:1607.00704 ancillary file (2016-07-11)
Supplement: Supplementary file 1 [file supplemental.pdf]

# Neutrino Flux Predictions for the Low Energy NuMI Beam – Supplemental

The MINERvA Collaboration

(Dated: May 13, 2016)

This supplemental contains fluxes for $\nu_\mu$, $\bar{\nu}_\mu$, $\nu_e$, and $\bar{\nu}_e$, for the standard NuMI low energy beam configurations: forward horn current (FHC), in which $\pi^+$ and $K^+$ were focused to produce a $\nu_\mu$ enriched beam; and reverse horn current (RHC), in which $\pi^-$ and $K^-$ were focused to produce a $\bar{\nu}_\mu$ enriched beam. In Fermilab's parlance the two beams are referred to as `LE010z185i` and `LE010z-185i`, respectively. They correspond to the major MINERvA run periods 1 and 13 (FNC) and 5 (RHC).

The fluxes are averaged over the MINERvA fiducial volume. The have been corrected using a suite of hadron production data as described in the accompanying paper. They have also been constrained using the $\nu e \to \nu e$ scattering measurement described briefly in the paper and also in `arXiv:1512.07699`.

**Flux text files:** These are files named like `neutrinoBEAM.txt`. The files contain the flux, uncertainties, and covariance matrix, with units of $\nu/m^2/POT$, in 0.5 GeV bins going up to 100 GeV. The first line in the file is the flux, the second is the uncertainty (200 numbers each), then there are 200 lines, each with 200 entries for the covariance matrix.

**Flux `ROOT` file:** The file `minerva_flux.root` contains histograms of the flux from 0-100 GeV (you may have to unzoom after drawing them) as well as the covariance and correlation matrices. The naming convention is `neutrino_beam` (flux histogram), `neutrino_beam_covmx` (covariance matrix), `neutrino_beam_cormx` (correlation matrix). Note, the histograms have been multiplied by a factor of $10^6$ for better display, making the units $\nu/m^2/10^6 POT$.

**`read_flux.py`:** A program which reads the flux text files and makes root histograms, including those displayed in this document.

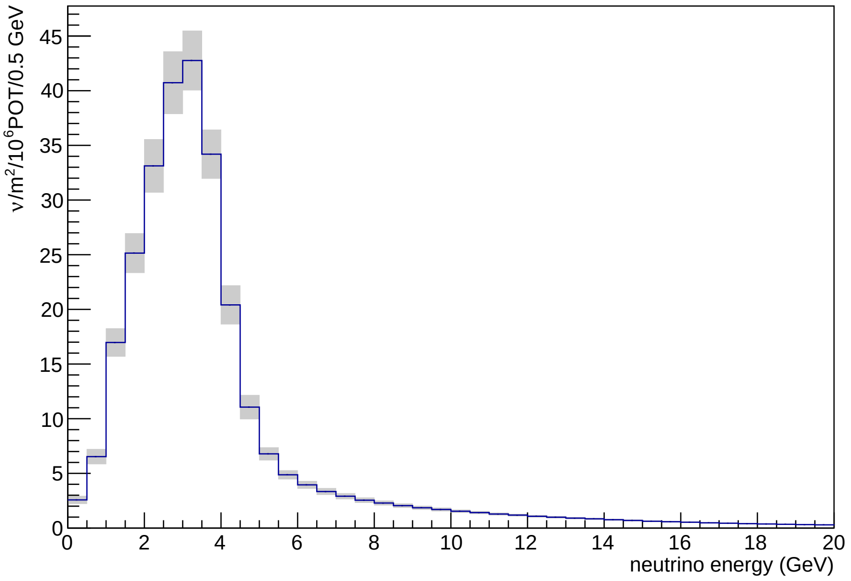


FIG. 1: The $\nu_\mu$ flux in units of $\nu/m^2/10^6 POT$ for the FHC beam.

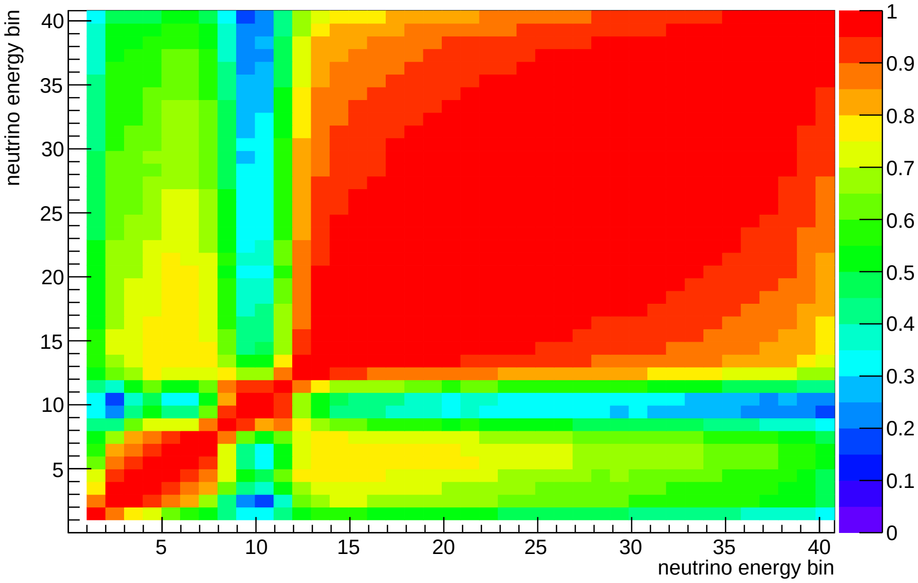


FIG. 2: The $\nu_\mu$ correlation matrix for the FHC beam.

TABLE I: The $\nu_\mu$ flux in units of $\nu/m^2/10^6 POT$ for the FHC beam.

| E (GeV) | $\phi$ | $\delta\phi$ (%) | E (GeV) | $\phi$ | $\delta\phi$ (%) |
|---|---|---|---|---|---|
| 0.0-0.5 | 2.57e+00 | 13.6 | 0.5-1.0 | 6.53e+00 | 10.3 |
| 1.0-1.5 | 1.70e+01 | 7.5 | 1.5-2.0 | 2.51e+01 | 7.1 |
| 2.0-2.5 | 3.31e+01 | 7.3 | 2.5-3.0 | 4.07e+01 | 7.0 |
| 3.0-3.5 | 4.28e+01 | 6.3 | 3.5-4.0 | 3.42e+01 | 6.5 |
| 4.0-4.5 | 2.04e+01 | 8.7 | 4.5-5.0 | 1.11e+01 | 9.8 |
| 5.0-5.5 | 6.79e+00 | 8.5 | 5.5-6.0 | 4.87e+00 | 8.1 |
| 6.0-6.5 | 3.95e+00 | 8.4 | 6.5-7.0 | 3.34e+00 | 8.7 |
| 7.0-7.5 | 2.91e+00 | 8.8 | 7.5-8.0 | 2.55e+00 | 8.8 |
| 8.0-8.5 | 2.29e+00 | 8.7 | 8.5-9.0 | 2.05e+00 | 8.7 |
| 9.0-9.5 | 1.85e+00 | 8.7 | 9.5-10.0 | 1.70e+00 | 8.6 |
| 10.0-10.5 | 1.54e+00 | 8.5 | 10.5-11.0 | 1.41e+00 | 8.4 |
| 11.0-11.5 | 1.28e+00 | 8.3 | 11.5-12.0 | 1.18e+00 | 8.3 |
| 12.0-12.5 | 1.07e+00 | 8.2 | 12.5-13.0 | 9.89e-01 | 8.2 |
| 13.0-13.5 | 9.06e-01 | 8.1 | 13.5-14.0 | 8.42e-01 | 8.0 |
| 14.0-14.5 | 7.61e-01 | 8.1 | 14.5-15.0 | 6.95e-01 | 8.0 |
| 15.0-15.5 | 6.19e-01 | 8.0 | 15.5-16.0 | 5.79e-01 | 8.0 |
| 16.0-16.5 | 5.32e-01 | 8.1 | 16.5-17.0 | 4.76e-01 | 8.0 |
| 17.0-17.5 | 4.40e-01 | 8.1 | 17.5-18.0 | 4.03e-01 | 8.1 |
| 18.0-18.5 | 3.71e-01 | 8.3 | 18.5-19.0 | 3.40e-01 | 8.4 |
| 19.0-19.5 | 3.17e-01 | 8.6 | 19.5-20.0 | 2.91e-01 | 8.9 |

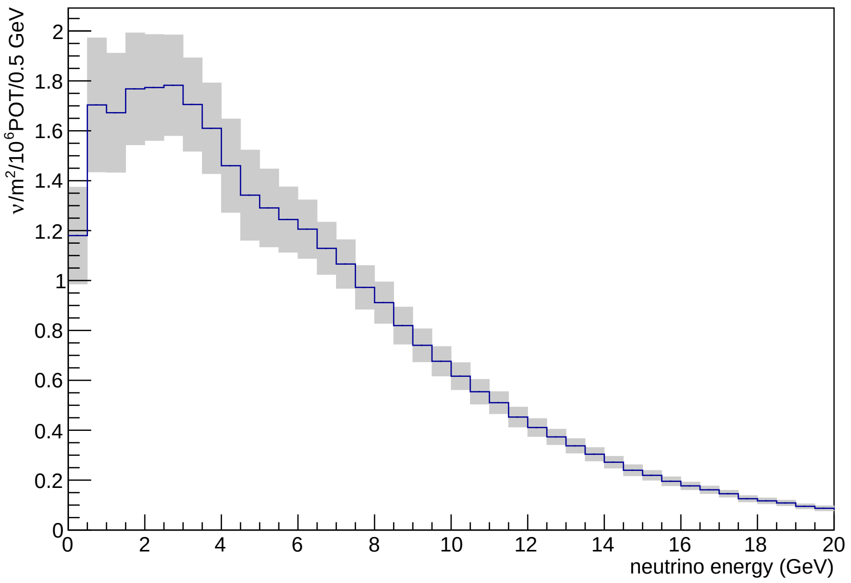


FIG. 3: The $\bar{\nu}_\mu$ flux in units of $\nu/m^2/10^6 POT$ for the FHC beam.

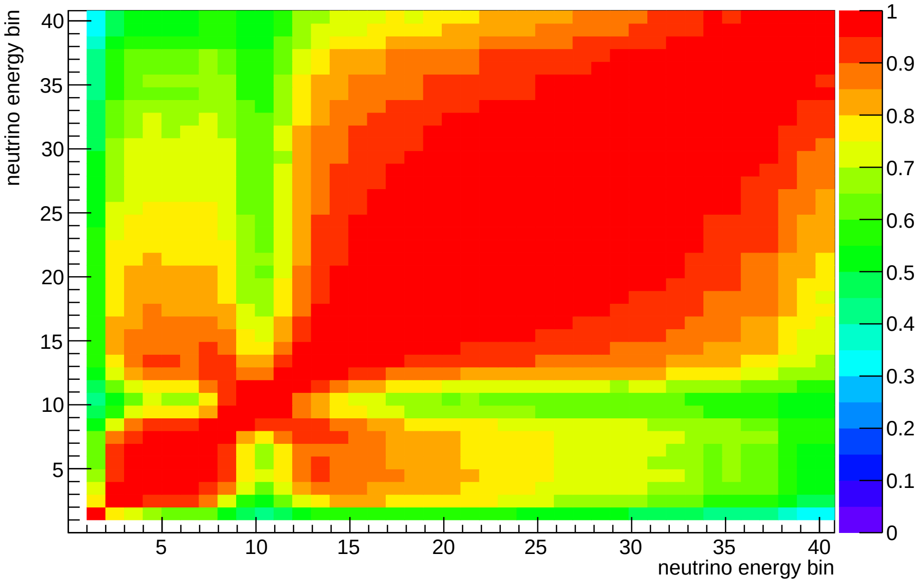


FIG. 4: The $\bar{\nu}_\mu$ correlation matrix for the FHC beam.

TABLE II: The $\bar{\nu}_\mu$ flux in units of $\nu/m^2/10^6POT$ for the FHC beam.

| E (GeV) | $\phi$ | $\delta\phi$ (%) | E (GeV) | $\phi$ | $\delta\phi$ (%) |
|---|---|---|---|---|---|
| 0.0-0.5 | 1.18e+00 | 16.5 | 0.5-1.0 | 1.70e+00 | 15.8 |
| 1.0-1.5 | 1.67e+00 | 14.3 | 1.5-2.0 | 1.77e+00 | 12.7 |
| 2.0-2.5 | 1.77e+00 | 12.0 | 2.5-3.0 | 1.78e+00 | 11.3 |
| 3.0-3.5 | 1.71e+00 | 11.0 | 3.5-4.0 | 1.61e+00 | 11.3 |
| 4.0-4.5 | 1.46e+00 | 12.8 | 4.5-5.0 | 1.34e+00 | 13.5 |
| 5.0-5.5 | 1.29e+00 | 12.1 | 5.5-6.0 | 1.24e+00 | 10.5 |
| 6.0-6.5 | 1.21e+00 | 9.8 | 6.5-7.0 | 1.13e+00 | 9.3 |
| 7.0-7.5 | 1.07e+00 | 9.2 | 7.5-8.0 | 9.72e-01 | 9.0 |
| 8.0-8.5 | 9.11e-01 | 9.1 | 8.5-9.0 | 8.19e-01 | 9.1 |
| 9.0-9.5 | 7.40e-01 | 9.0 | 9.5-10.0 | 6.76e-01 | 8.8 |
| 10.0-10.5 | 6.17e-01 | 8.8 | 10.5-11.0 | 5.54e-01 | 9.0 |
| 11.0-11.5 | 5.10e-01 | 8.7 | 11.5-12.0 | 4.53e-01 | 8.9 |
| 12.0-12.5 | 4.11e-01 | 8.8 | 12.5-13.0 | 3.73e-01 | 8.4 |
| 13.0-13.5 | 3.37e-01 | 8.7 | 13.5-14.0 | 3.04e-01 | 8.9 |
| 14.0-14.5 | 2.72e-01 | 8.8 | 14.5-15.0 | 2.40e-01 | 9.4 |
| 15.0-15.5 | 2.19e-01 | 9.1 | 15.5-16.0 | 1.95e-01 | 9.3 |
| 16.0-16.5 | 1.77e-01 | 8.9 | 16.5-17.0 | 1.61e-01 | 9.6 |
| 17.0-17.5 | 1.45e-01 | 9.7 | 17.5-18.0 | 1.26e-01 | 10.3 |
| 18.0-18.5 | 1.17e-01 | 10.2 | 18.5-19.0 | 1.09e-01 | 10.5 |
| 19.0-19.5 | 9.50e-02 | 10.8 | 19.5-20.0 | 8.71e-02 | 11.8 |

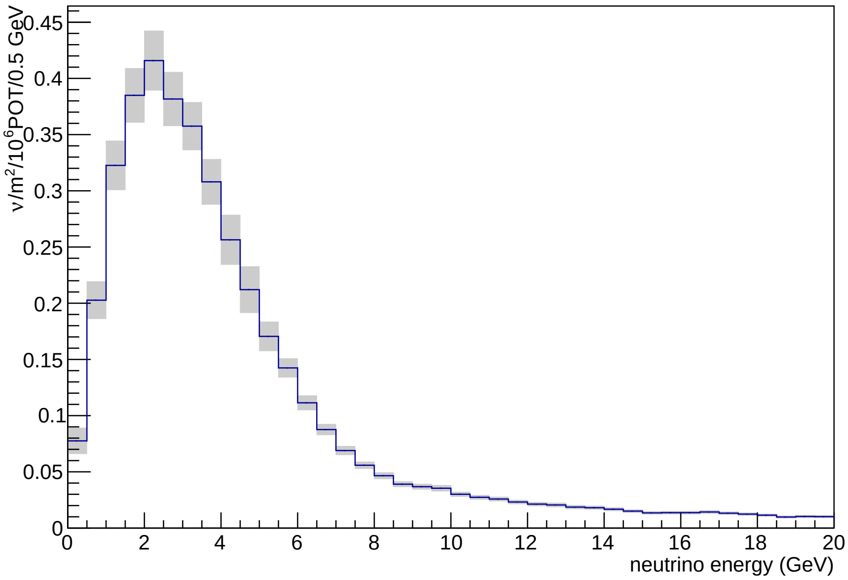


FIG. 5: The $\nu_e$ flux in units of $\nu/m^2/10^6POT$ for the FHC beam.

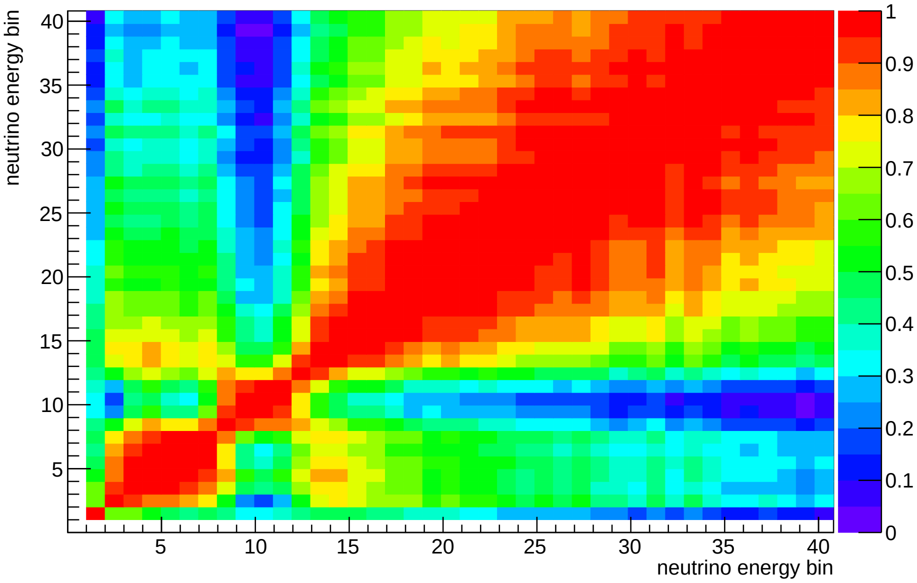


FIG. 6: The $\nu_e$ correlation matrix for the FHC beam.

TABLE III: The $\nu_e$ flux in units of $\nu/m^2/10^6 POT$ for the FHC beam.

| E (GeV) | $\phi$ | $\delta\phi$ (%) | E (GeV) | $\phi$ | $\delta\phi$ (%) |
|---|---|---|---|---|---|
| 0.0-0.5 | 7.75e-02 | 14.8 | 0.5-1.0 | 2.03e-01 | 8.2 |
| 1.0-1.5 | 3.23e-01 | 6.8 | 1.5-2.0 | 3.85e-01 | 6.2 |
| 2.0-2.5 | 4.16e-01 | 6.4 | 2.5-3.0 | 3.82e-01 | 6.3 |
| 3.0-3.5 | 3.58e-01 | 5.9 | 3.5-4.0 | 3.08e-01 | 6.5 |
| 4.0-4.5 | 2.56e-01 | 8.6 | 4.5-5.0 | 2.12e-01 | 9.7 |
| 5.0-5.5 | 1.71e-01 | 7.6 | 5.5-6.0 | 1.42e-01 | 5.9 |
| 6.0-6.5 | 1.11e-01 | 5.7 | 6.5-7.0 | 8.76e-02 | 5.4 |
| 7.0-7.5 | 6.89e-02 | 5.6 | 7.5-8.0 | 5.58e-02 | 5.4 |
| 8.0-8.5 | 4.66e-02 | 6.1 | 8.5-9.0 | 3.90e-02 | 6.1 |
| 9.0-9.5 | 3.68e-02 | 6.5 | 9.5-10.0 | 3.54e-02 | 7.4 |
| 10.0-10.5 | 3.00e-02 | 6.8 | 10.5-11.0 | 2.73e-02 | 7.0 |
| 11.0-11.5 | 2.58e-02 | 7.2 | 11.5-12.0 | 2.32e-02 | 7.5 |
| 12.0-12.5 | 2.13e-02 | 7.8 | 12.5-13.0 | 2.05e-02 | 8.6 |
| 13.0-13.5 | 1.86e-02 | 8.9 | 13.5-14.0 | 1.81e-02 | 8.6 |
| 14.0-14.5 | 1.67e-02 | 8.9 | 14.5-15.0 | 1.51e-02 | 9.3 |
| 15.0-15.5 | 1.35e-02 | 9.6 | 15.5-16.0 | 1.37e-02 | 9.4 |
| 16.0-16.5 | 1.37e-02 | 9.8 | 16.5-17.0 | 1.43e-02 | 9.6 |
| 17.0-17.5 | 1.32e-02 | 9.6 | 17.5-18.0 | 1.24e-02 | 10.3 |
| 18.0-18.5 | 1.15e-02 | 9.9 | 18.5-19.0 | 9.82e-03 | 10.9 |
| 19.0-19.5 | 1.03e-02 | 10.7 | 19.5-20.0 | 1.02e-02 | 11.3 |

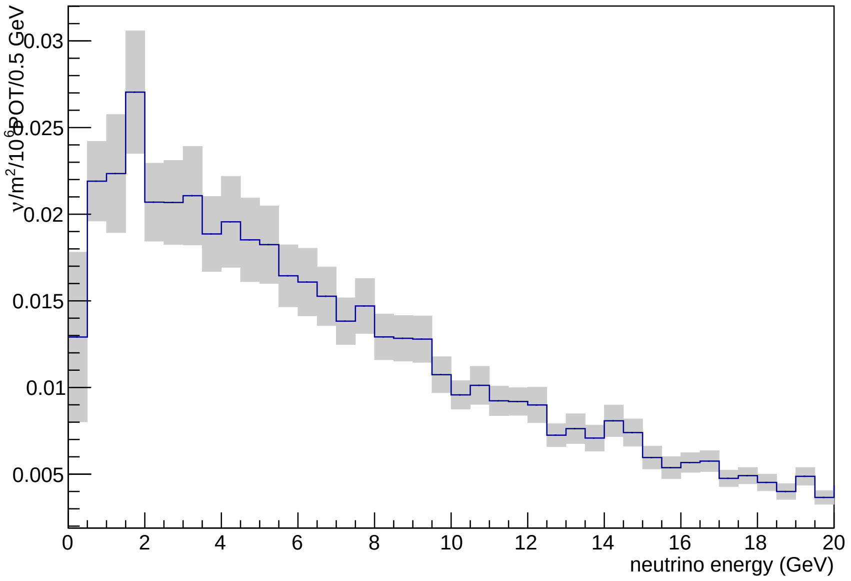


FIG. 7: The $\bar{\nu}_e$ flux in units of $\nu/m^2/10^6 POT$ for the FHC beam.

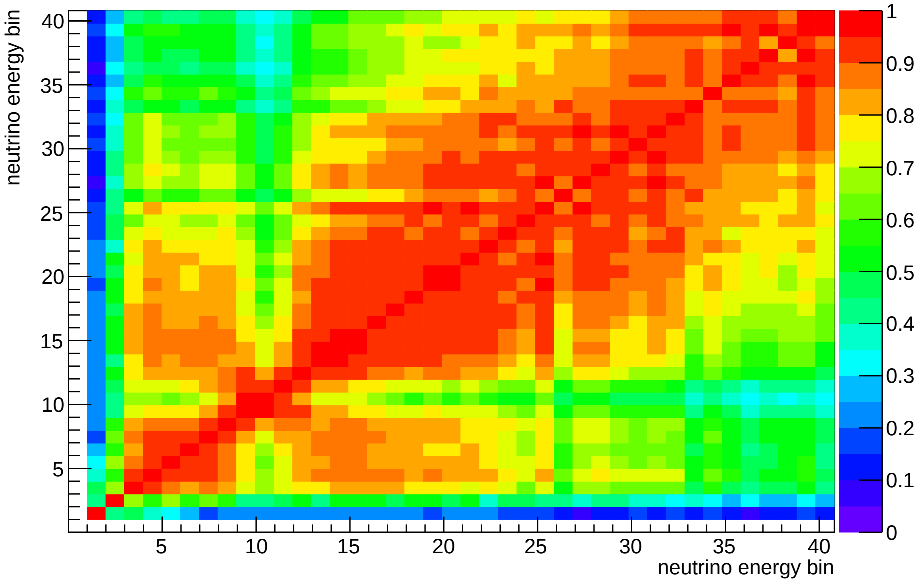


FIG. 8: The $\bar{\nu}_e$ correlation matrix for the FHC beam.

TABLE IV: The $\bar{\nu}_e$ flux in units of $\nu/m^2/10^6 POT$ for the FHC beam.

| E (GeV) | $\phi$ | $\delta\phi$ (%) | E (GeV) | $\phi$ | $\delta\phi$ (%) |
|---|---|---|---|---|---|
| 0.0-0.5 | 1.29e-02 | 37.9 | 0.5-1.0 | 2.19e-02 | 10.5 |
| 1.0-1.5 | 2.23e-02 | 15.3 | 1.5-2.0 | 2.70e-02 | 13.1 |
| 2.0-2.5 | 2.07e-02 | 10.9 | 2.5-3.0 | 2.07e-02 | 11.7 |
| 3.0-3.5 | 2.11e-02 | 13.5 | 3.5-4.0 | 1.89e-02 | 11.5 |
| 4.0-4.5 | 1.96e-02 | 13.4 | 4.5-5.0 | 1.85e-02 | 13.0 |
| 5.0-5.5 | 1.82e-02 | 12.3 | 5.5-6.0 | 1.64e-02 | 10.9 |
| 6.0-6.5 | 1.61e-02 | 12.1 | 6.5-7.0 | 1.53e-02 | 11.1 |
| 7.0-7.5 | 1.38e-02 | 9.8 | 7.5-8.0 | 1.47e-02 | 10.8 |
| 8.0-8.5 | 1.29e-02 | 10.2 | 8.5-9.0 | 1.28e-02 | 10.3 |
| 9.0-9.5 | 1.28e-02 | 10.5 | 9.5-10.0 | 1.07e-02 | 9.7 |
| 10.0-10.5 | 9.57e-03 | 8.6 | 10.5-11.0 | 1.01e-02 | 10.8 |
| 11.0-11.5 | 9.23e-03 | 9.3 | 11.5-12.0 | 9.19e-03 | 8.7 |
| 12.0-12.5 | 8.99e-03 | 11.4 | 12.5-13.0 | 7.25e-03 | 9.1 |
| 13.0-13.5 | 7.63e-03 | 11.3 | 13.5-14.0 | 7.08e-03 | 10.6 |
| 14.0-14.5 | 8.08e-03 | 11.3 | 14.5-15.0 | 7.40e-03 | 10.7 |
| 15.0-15.5 | 5.96e-03 | 11.1 | 15.5-16.0 | 5.37e-03 | 11.9 |
| 16.0-16.5 | 5.67e-03 | 10.0 | 16.5-17.0 | 5.75e-03 | 10.5 |
| 17.0-17.5 | 4.76e-03 | 9.9 | 17.5-18.0 | 4.91e-03 | 9.6 |
| 18.0-18.5 | 4.52e-03 | 10.7 | 18.5-19.0 | 4.00e-03 | 11.5 |
| 19.0-19.5 | 4.87e-03 | 10.5 | 19.5-20.0 | 3.66e-03 | 10.9 |

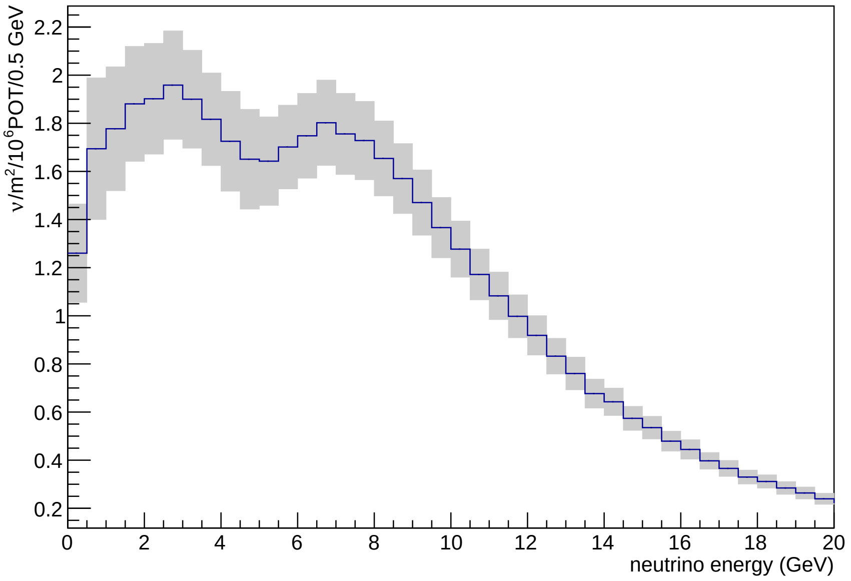


FIG. 9: The $\nu_\mu$ flux in units of $\nu/m^2/10^6 POT$ for the RHC beam.

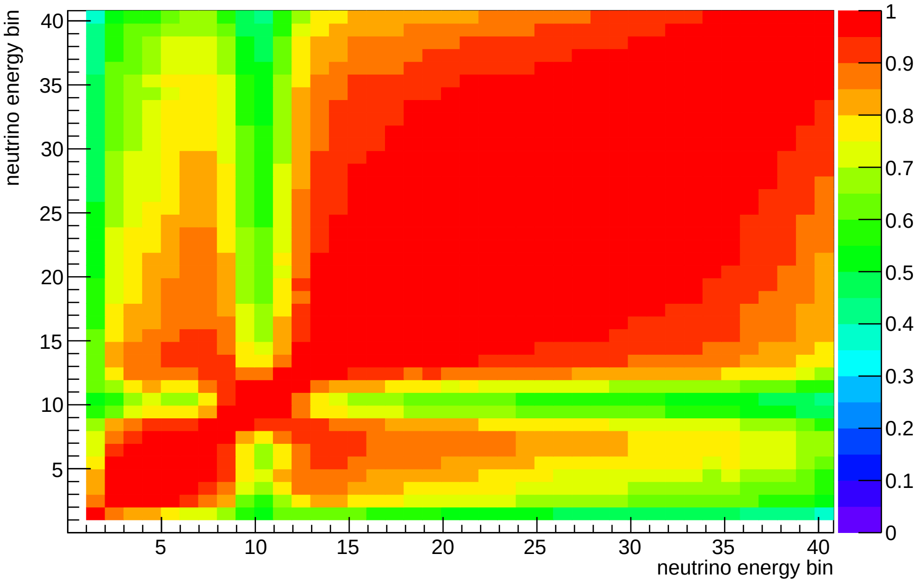


FIG. 10: The $\nu_\mu$ correlation matrix for the RHC beam.

TABLE V: The $\nu_\mu$ flux in units of $\nu/m^2/10^6 POT$ for the RHC beam.

| E (GeV) | $\phi$ | $\delta\phi$ (%) | E (GeV) | $\phi$ | $\delta\phi$ (%) |
|---|---|---|---|---|---|
| 0.0-0.5 | 1.26e+00 | 16.2 | 0.5-1.0 | 1.69e+00 | 17.4 |
| 1.0-1.5 | 1.78e+00 | 14.5 | 1.5-2.0 | 1.88e+00 | 12.7 |
| 2.0-2.5 | 1.90e+00 | 12.1 | 2.5-3.0 | 1.96e+00 | 11.5 |
| 3.0-3.5 | 1.90e+00 | 10.7 | 3.5-4.0 | 1.82e+00 | 10.6 |
| 4.0-4.5 | 1.73e+00 | 12.0 | 4.5-5.0 | 1.65e+00 | 12.6 |
| 5.0-5.5 | 1.64e+00 | 11.2 | 5.5-6.0 | 1.70e+00 | 10.2 |
| 6.0-6.5 | 1.75e+00 | 10.1 | 6.5-7.0 | 1.80e+00 | 9.8 |
| 7.0-7.5 | 1.76e+00 | 9.6 | 7.5-8.0 | 1.73e+00 | 9.4 |
| 8.0-8.5 | 1.65e+00 | 9.4 | 8.5-9.0 | 1.57e+00 | 9.3 |
| 9.0-9.5 | 1.47e+00 | 9.2 | 9.5-10.0 | 1.37e+00 | 9.2 |
| 10.0-10.5 | 1.28e+00 | 9.1 | 10.5-11.0 | 1.17e+00 | 9.0 |
| 11.0-11.5 | 1.08e+00 | 9.1 | 11.5-12.0 | 9.98e-01 | 8.9 |
| 12.0-12.5 | 9.19e-01 | 8.9 | 12.5-13.0 | 8.32e-01 | 8.9 |
| 13.0-13.5 | 7.60e-01 | 8.9 | 13.5-14.0 | 6.77e-01 | 8.9 |
| 14.0-14.5 | 6.43e-01 | 8.8 | 14.5-15.0 | 5.74e-01 | 8.7 |
| 15.0-15.5 | 5.35e-01 | 8.8 | 15.5-16.0 | 4.79e-01 | 8.7 |
| 16.0-16.5 | 4.45e-01 | 9.1 | 16.5-17.0 | 3.97e-01 | 8.8 |
| 17.0-17.5 | 3.66e-01 | 9.1 | 17.5-18.0 | 3.30e-01 | 8.8 |
| 18.0-18.5 | 3.11e-01 | 8.9 | 18.5-19.0 | 2.85e-01 | 9.3 |
| 19.0-19.5 | 2.64e-01 | 9.4 | 19.5-20.0 | 2.39e-01 | 9.6 |

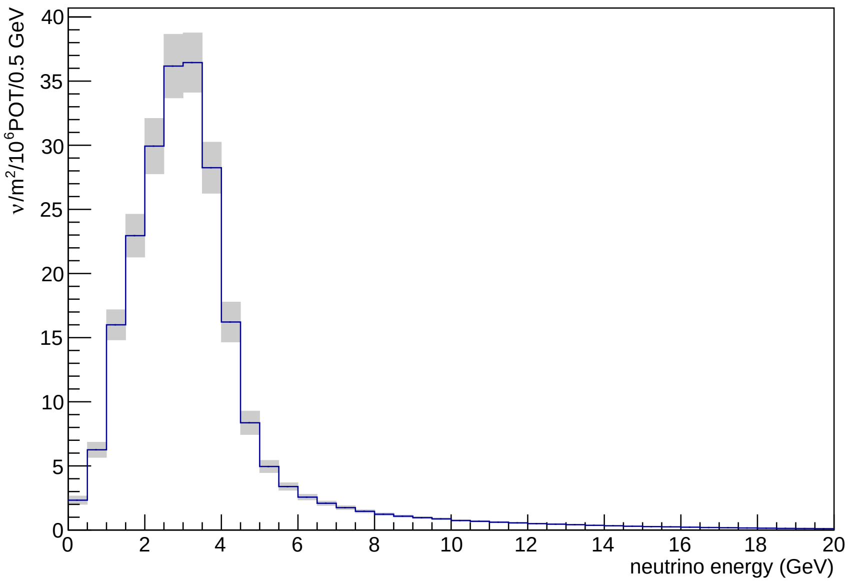


FIG. 11: The $\bar{\nu}_\mu$ flux in units of $\nu/m^2/10^6 POT$ for the RHC beam.

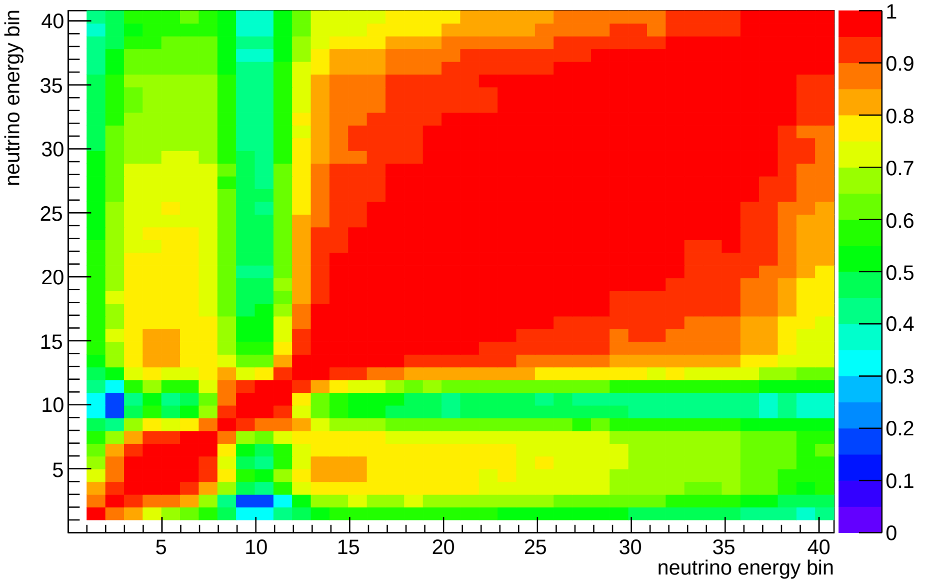


FIG. 12: The $\bar{\nu}_\mu$ correlation matrix for the RHC beam.

TABLE VI: The $\bar{\nu}_\mu$ flux in units of $\nu/m^2/10^6 POT$ for the RHC beam.

| E (GeV) | $\phi$ | $\delta\phi$ (%) | E (GeV) | $\phi$ | $\delta\phi$ (%) |
|---|---|---|---|---|---|
| 0.0-0.5 | 2.33e+00 | 14.2 | 0.5-1.0 | 6.26e+00 | 9.5 |
| 1.0-1.5 | 1.60e+01 | 7.4 | 1.5-2.0 | 2.30e+01 | 7.3 |
| 2.0-2.5 | 2.99e+01 | 7.2 | 2.5-3.0 | 3.62e+01 | 6.9 |
| 3.0-3.5 | 3.64e+01 | 6.3 | 3.5-4.0 | 2.82e+01 | 7.1 |
| 4.0-4.5 | 1.62e+01 | 9.6 | 4.5-5.0 | 8.36e+00 | 11.0 |
| 5.0-5.5 | 4.95e+00 | 9.7 | 5.5-6.0 | 3.39e+00 | 8.7 |
| 6.0-6.5 | 2.57e+00 | 8.6 | 6.5-7.0 | 2.09e+00 | 8.4 |
| 7.0-7.5 | 1.75e+00 | 8.5 | 7.5-8.0 | 1.46e+00 | 8.5 |
| 8.0-8.5 | 1.23e+00 | 8.5 | 8.5-9.0 | 1.08e+00 | 8.4 |
| 9.0-9.5 | 9.67e-01 | 8.1 | 9.5-10.0 | 8.70e-01 | 8.3 |
| 10.0-10.5 | 7.42e-01 | 8.3 | 10.5-11.0 | 6.81e-01 | 8.1 |
| 11.0-11.5 | 6.11e-01 | 8.1 | 11.5-12.0 | 5.58e-01 | 8.0 |
| 12.0-12.5 | 4.99e-01 | 8.1 | 12.5-13.0 | 4.58e-01 | 7.9 |
| 13.0-13.5 | 4.17e-01 | 8.1 | 13.5-14.0 | 3.67e-01 | 7.9 |
| 14.0-14.5 | 3.32e-01 | 7.7 | 14.5-15.0 | 2.96e-01 | 8.3 |
| 15.0-15.5 | 2.68e-01 | 8.3 | 15.5-16.0 | 2.47e-01 | 8.3 |
| 16.0-16.5 | 2.23e-01 | 8.5 | 16.5-17.0 | 1.98e-01 | 8.5 |
| 17.0-17.5 | 1.80e-01 | 8.4 | 17.5-18.0 | 1.61e-01 | 8.7 |
| 18.0-18.5 | 1.47e-01 | 8.9 | 18.5-19.0 | 1.29e-01 | 9.5 |
| 19.0-19.5 | 1.20e-01 | 10.1 | 19.5-20.0 | 1.08e-01 | 10.5 |

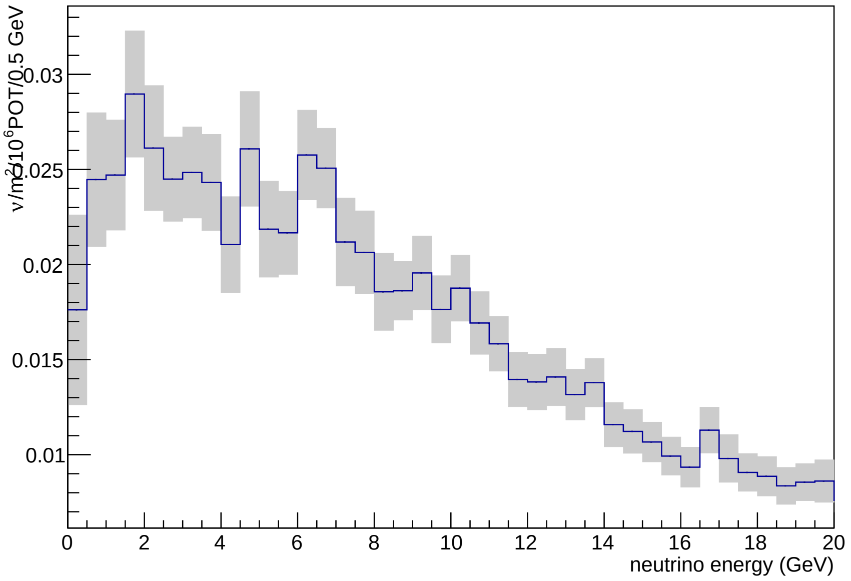


FIG. 13: The $\nu_e$ flux in units of $\nu/m^2/10^6 POT$ for the RHC beam.

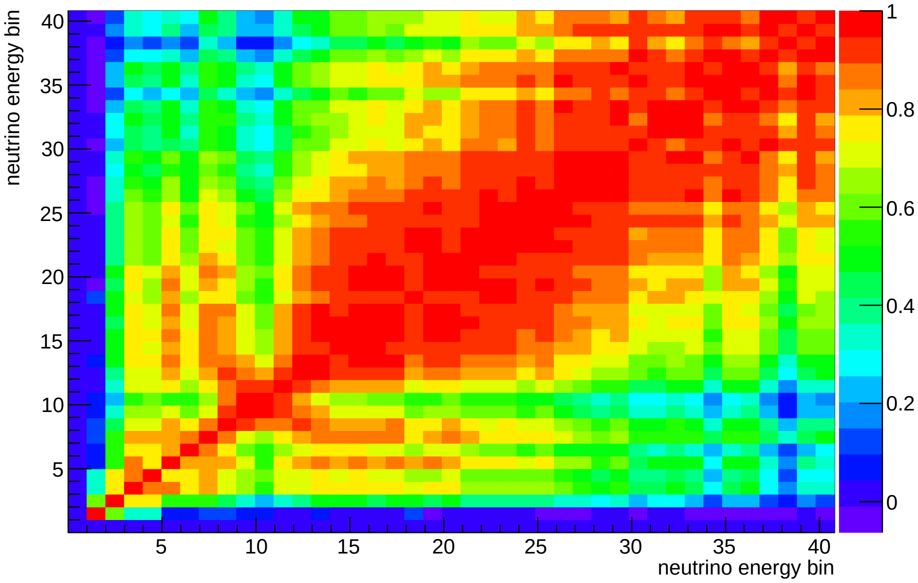


FIG. 14: The $\nu_e$ correlation matrix for the RHC beam.

TABLE VII: The $\nu_e$ flux in units of $\nu/m^2/10^6 POT$ for the RHC beam.

| E (GeV) | $\phi$ | $\delta\phi$ (%) | E (GeV) | $\phi$ | $\delta\phi$ (%) |
|---|---|---|---|---|---|
| 0.0-0.5 | 1.76e-02 | 28.3 | 0.5-1.0 | 2.45e-02 | 14.4 |
| 1.0-1.5 | 2.47e-02 | 11.7 | 1.5-2.0 | 2.90e-02 | 11.5 |
| 2.0-2.5 | 2.61e-02 | 12.6 | 2.5-3.0 | 2.45e-02 | 9.1 |
| 3.0-3.5 | 2.48e-02 | 9.6 | 3.5-4.0 | 2.43e-02 | 10.4 |
| 4.0-4.5 | 2.11e-02 | 12.0 | 4.5-5.0 | 2.61e-02 | 11.6 |
| 5.0-5.5 | 2.19e-02 | 11.6 | 5.5-6.0 | 2.17e-02 | 10.1 |
| 6.0-6.5 | 2.58e-02 | 9.2 | 6.5-7.0 | 2.51e-02 | 8.4 |
| 7.0-7.5 | 2.12e-02 | 10.9 | 7.5-8.0 | 2.06e-02 | 10.6 |
| 8.0-8.5 | 1.86e-02 | 10.9 | 8.5-9.0 | 1.86e-02 | 8.3 |
| 9.0-9.5 | 1.96e-02 | 9.9 | 9.5-10.0 | 1.76e-02 | 10.0 |
| 10.0-10.5 | 1.88e-02 | 9.3 | 10.5-11.0 | 1.69e-02 | 9.7 |
| 11.0-11.5 | 1.58e-02 | 9.1 | 11.5-12.0 | 1.40e-02 | 10.3 |
| 12.0-12.5 | 1.38e-02 | 10.6 | 12.5-13.0 | 1.41e-02 | 10.7 |
| 13.0-13.5 | 1.32e-02 | 10.2 | 13.5-14.0 | 1.38e-02 | 9.2 |
| 14.0-14.5 | 1.16e-02 | 10.1 | 14.5-15.0 | 1.12e-02 | 10.3 |
| 15.0-15.5 | 1.07e-02 | 9.8 | 15.5-16.0 | 9.93e-03 | 10.1 |
| 16.0-16.5 | 9.34e-03 | 11.3 | 16.5-17.0 | 1.13e-02 | 10.7 |
| 17.0-17.5 | 9.80e-03 | 12.8 | 17.5-18.0 | 9.07e-03 | 10.9 |
| 18.0-18.5 | 8.86e-03 | 11.7 | 18.5-19.0 | 8.36e-03 | 11.6 |
| 19.0-19.5 | 8.56e-03 | 11.4 | 19.5-20.0 | 8.61e-03 | 13.0 |

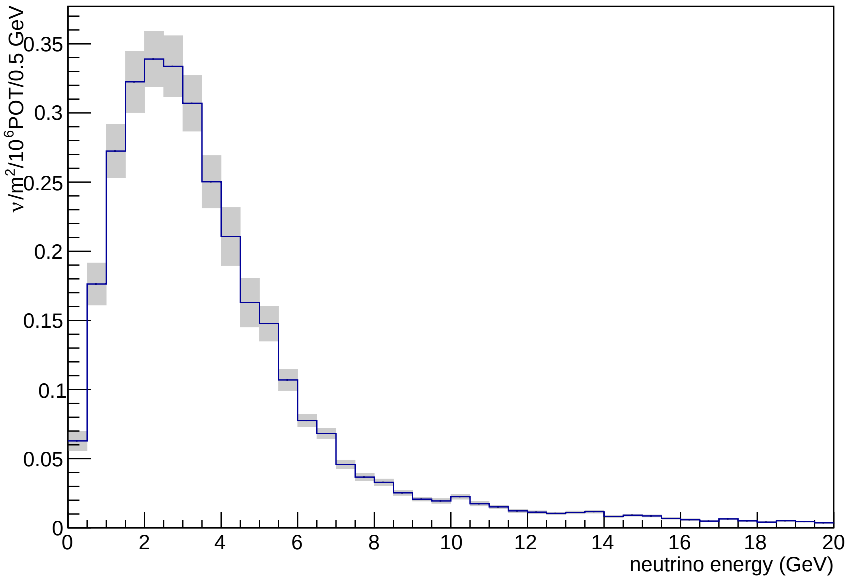


FIG. 15: The $\bar{\nu}_e$ flux in units of $\nu/m^2/10^6 POT$ for the RHC beam.

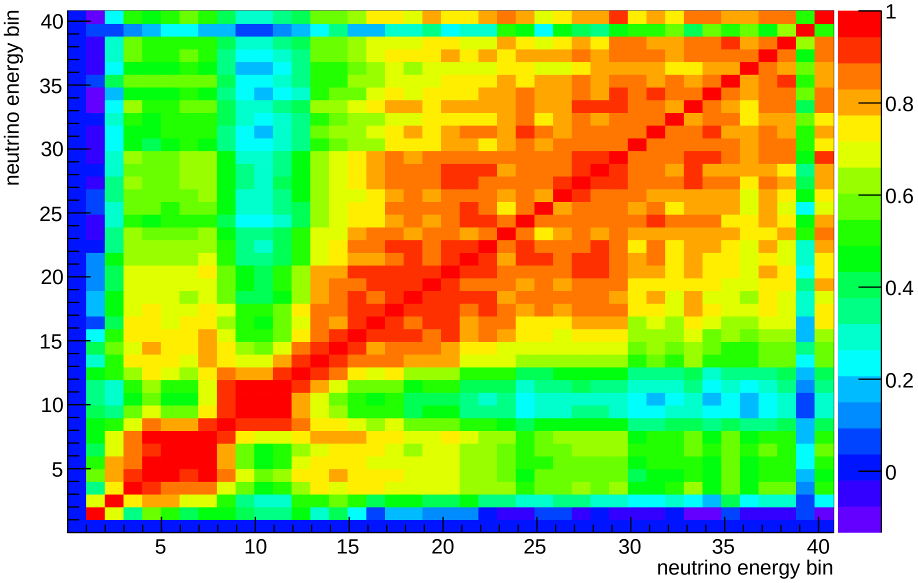


FIG. 16: The $\bar{\nu}_e$ correlation matrix for the RHC beam.

TABLE VIII: The $\bar{\nu}_e$ flux in units of $\nu/m^2/10^6 POT$ for the RHC beam.

| E (GeV) | $\phi$ | $\delta\phi$ (%) | E (GeV) | $\phi$ | $\delta\phi$ (%) |
|---|---|---|---|---|---|
| 0.0-0.5 | 6.28e-02 | 11.3 | 0.5-1.0 | 1.76e-01 | 8.7 |
| 1.0-1.5 | 2.72e-01 | 7.1 | 1.5-2.0 | 3.22e-01 | 6.9 |
| 2.0-2.5 | 3.39e-01 | 6.0 | 2.5-3.0 | 3.34e-01 | 6.6 |
| 3.0-3.5 | 3.07e-01 | 6.6 | 3.5-4.0 | 2.50e-01 | 7.6 |
| 4.0-4.5 | 2.11e-01 | 10.0 | 4.5-5.0 | 1.63e-01 | 10.9 |
| 5.0-5.5 | 1.48e-01 | 8.6 | 5.5-6.0 | 1.07e-01 | 7.2 |
| 6.0-6.5 | 7.75e-02 | 5.7 | 6.5-7.0 | 6.82e-02 | 5.3 |
| 7.0-7.5 | 4.58e-02 | 7.0 | 7.5-8.0 | 3.67e-02 | 7.7 |
| 8.0-8.5 | 3.29e-02 | 7.3 | 8.5-9.0 | 2.53e-02 | 7.2 |
| 9.0-9.5 | 2.08e-02 | 7.0 | 9.5-10.0 | 1.94e-02 | 8.9 |
| 10.0-10.5 | 2.25e-02 | 8.1 | 10.5-11.0 | 1.74e-02 | 9.4 |
| 11.0-11.5 | 1.51e-02 | 7.2 | 11.5-12.0 | 1.22e-02 | 9.3 |
| 12.0-12.5 | 1.14e-02 | 8.7 | 12.5-13.0 | 1.05e-02 | 8.8 |
| 13.0-13.5 | 1.11e-02 | 10.1 | 13.5-14.0 | 1.17e-02 | 9.4 |
| 14.0-14.5 | 8.22e-03 | 10.3 | 14.5-15.0 | 9.14e-03 | 8.3 |
| 15.0-15.5 | 8.59e-03 | 9.4 | 15.5-16.0 | 6.84e-03 | 9.0 |
| 16.0-16.5 | 5.83e-03 | 13.0 | 16.5-17.0 | 4.87e-03 | 9.6 |
| 17.0-17.5 | 6.44e-03 | 10.3 | 17.5-18.0 | 5.04e-03 | 9.2 |
| 18.0-18.5 | 4.13e-03 | 12.1 | 18.5-19.0 | 5.13e-03 | 10.5 |
| 19.0-19.5 | 4.48e-03 | 8.2 | 19.5-20.0 | 3.62e-03 | 11.9 |
